# Supplementary material for: APITestGenie: Automated API Test Generation through Generative AI
Source: arXiv:2409.03838 source file (2024-09-05)
Supplement: Supplementary file 1 [file appendix1.tex]

\chapter{GPT Generation TypeScript Sort Array}\label{apx:gptSortArray}

Certainly! Below is a sample TypeScript test using Jest and the Axios library to test an API endpoint that sorts a list of integers. This test assumes that you have a backend service with an endpoint `/sort-integers` that accepts an array of integers and returns a sorted array.  
   
First, make sure you have the necessary packages installed:  

\begin{verbatim}
```bash  
npm install jest @types/jest ts-jest axios @types/axios  
```  
\end{verbatim}
   
Then, create a file `sortIntegers.test.ts` with the following content:  

\begin{lstlisting}[style=python]
```typescript  
// sortIntegers.test.ts  
   
import axios from 'axios';  
import { AxiosResponse } from 'axios';  
   
// Mocking Axios to prevent actual HTTP requests during tests  
jest.mock('axios');  
const mockedAxios = axios as jest.Mocked<typeof axios>;  
   
// Test suite for the sort-integers endpoint  
describe('sortIntegers API endpoint', () => {  
  it('should sort an array of integers', async () => {  
    // The input and expected output  
    const unsortedArray = [34, 7, 23, 32, 5, 62];  
    const sortedArray = [5, 7, 23, 32, 34, 62];  
  
    // Mocking the Axios response  
    const mockResponse: AxiosResponse = {  
      data: sortedArray,  
      status: 200,  
      statusText: 'OK',  
      headers: {},  
      config: {},  
    };  
  
    mockedAxios.post.mockResolvedValueOnce(mockResponse);  
  
    // Perform the API call to the hypothetical endpoint  
    const response = await axios.post('/sort-integers', { integers: unsortedArray });  
  
    // Expectations  
    expect(mockedAxios.post).toHaveBeenCalledWith('/sort-integers', { integers: unsortedArray });  
    expect(response.data).toEqual(sortedArray);  
  });  
});  
```  
\end{lstlisting}

To run this test, you need to configure Jest to work with TypeScript. Create a `jest.config.js` file with the following content:  

\begin{lstlisting}[style=python]
```javascript  
// jest.config.js  
   
module.exports = {  
  preset: 'ts-jest',  
  testEnvironment: 'node',  
};  
```  
\end{lstlisting}
   
Now you can run your tests using the following command:  

\begin{spverbatim}
```bash  
npx jest sortIntegers.test.ts  
```  
\end{spverbatim}

This will execute your test, and you should see output indicating whether the test passed or failed. Remember that the actual implementation of the sorting endpoint is not provided here, so you'll need to have an API endpoint running that can handle the POST request and return a sorted array for this test to pass.
