# Supplementary material for: APITestGenie: Automated API Test Generation through Generative AI
Source: arXiv:2409.03838 source file (2024-09-05)
Supplement: Supplementary file 2 [file appendix2.tex]

\chapter{Progressive run generations}\label{apx:progressiveRun}

\section{Progressive run 1º Generation}

REQUIREMENT: As a user I want to retrieve all the countries where the service is available.

ENDPOINTS: The relevant endpoint to test this business requirement is:

1) GET /otd\censor{/country-groups}
    - Description: Returns Country Groups for which OTD are available.
    - Response: A list of strings representing country group names.

TEST:
\begin{lstlisting}[style=python]
```typescript

import axios from 'axios';

// Define the base URL and API key from the environment variables.
const baseURL = process.env.UCP_BASE_ENDPOINT;
const apiKey = process.env.UCP_X_API_KEY;

describe('Retrieve available country groups', () => {
  test('It should return an array of country groups', async () => {
    const response = await axios.get(`${baseURL}/otd#\censor{/country-groups}#`, {
      headers: { #\censor{'x-api-key'}#: apiKey }
    });

    // Verify the request was successful
    expect(response.status).toBe(200);

    // Verify that the data is an array
    expect(Array.isArray(response.data)).toBe(true);

    // Additional check: verify that array contains string values (assuming country groups are strings)
    if (response.data.length > 0) {
      expect(typeof response.data[0]).toBe('string');
    }
  });

  test('It should require an API key and fail without it', async () => {
    try {
      await axios.get(`${baseURL}/otd#\censor{/country-groups}#`);
    } catch (error) {
      expect(error.response.status).toBe(401);
    }
  });
});
```
\end{lstlisting}

\section{Progressive run 2º Generation}

REQUIREMENT: As a user I want to retrieve all the available ag-models in the eu27+ country so that I can know which vehicles are available.

ENDPOINTS: The endpoint for retrieving available AG-models within a specific country group is a GET request to: `/otd\censor{/country-groups/{countryGroup}/ag-models}`

- Request: The request takes a countryGroup as a path parameter.

- Response: The response should be an array of strings representing AG-model codes.

TEST:
\begin{lstlisting}[style=python]
```typescript

import axios from 'axios';

// Test suite for AG-models retrieval
describe('Retrieve available AG-models for eu27+ country group', () => {
  const countryGroup = 'eu27+';
  const baseUrl = process.env.UCP_BASE_ENDPOINT;
  const apiKey = process.env.UCP_X_API_KEY;
  const agModelsEndpoint = `/otd#\censor{/country-groups/\${countryGroup}/ag-models}#`;

  test(`should retrieve a list of all AG-models in the "${countryGroup}" country group`, async () => {
    // Setup
    const fullUrl = `${baseUrl}${agModelsEndpoint}`;
    const config = {
      headers: {
        #\censor{'x-api-key'}#: apiKey,
      },
    };

    // Execution
    const response = await axios.get(fullUrl, config);

    // Validations
    expect(response.status).toBe(200);
    expect(Array.isArray(response.data)).toBe(true);
    response.data.forEach(modelCode => {
      expect(typeof modelCode).toBe('string');
    });

    // If additional information is needed about an AG-model, validate structure and type here.
    // For example, if each AG-model should match a specific format or pattern, you could add:
    // response.data.forEach(modelCode => {
    //   expect(modelCode).toMatch(someRegularExpression);
    // });
  });

  // Additional tests for error scenarios, like unauthorized access, bad request, etc. could be included here.
});
```
\end{lstlisting}

\section{Progressive run 3º Generation}

REQUIREMENT: As a user I want to retrieve all the existing country codes then select one so that I can retrieve all the available ag-models for the country so that I can know which vehicles are available.

ENDPOINTS:

1) **Retrieve Country Groups**
    - GET /otd\censor{/country-groups}
    - Response: Array of strings representing country codes (e.g., ['usa-kanada', 'japan', 'ece', 'china']).

2) **Retrieve AG-Models for a Country**
    -   GET /otd\censor{/country-groups/{countryGroup}/ag-models}
    -   Response: Array of strings representing AG-Models (e.g., [\censor{'0J53', '2H52', 'JR32', '7C62', '4Y91', '4Y92'}]).

TEST:
\begin{lstlisting}[style=python]
```typescript
import axios from 'axios';

describe('Retrieve AG-Models for a selected Country Code', () => {
  const apiKey = process.env.UCP_X_API_KEY;
  const baseUrl = process.env.UCP_BASE_ENDPOINT;
  let selectedCountryCode = '';
  let availableAGModels = [];

  test('Retrieve available country codes', async () => {
    const response = await axios.get(`\${baseUrl}/otd#\censor{/country-groups}#`, {
      headers: { #\censor{'x-api-key'}#: apiKey },
    });

    // Assert the response contains an array of country codes
    expect(response.status).toBe(200);
    expect(Array.isArray(response.data)).toBeTruthy();
    expect(response.data.length).toBeGreaterThan(0);

    // Store a selected country code for the next test
    selectedCountryCode = response.data[0];
  });

  test('Retrieve available AG-Models for a country code', async () => {
    // Ensure there is a country code selected from the previous test
    expect(selectedCountryCode).toBeTruthy();

    const response = await axios.get(`${baseUrl}/otd#\censor{/country-groups/}#${ selectedCountryCode}/ag-models`, {
      headers: { #\censor{'x-api-key'}#: apiKey },
    });

    // Assert the response contains an array of AG-Models
    expect(response.status).toBe(200);
    expect(Array.isArray(response.data)).toBeTruthy();
    expect(response.data.length).toBeGreaterThan(0);

    // Store the AG-Models for potential further tests or use
    availableAGModels = response.data;
  });

  // Additional tests can be added here to continue interacting with the API
  // and to cover more scenarios according to the requirements
});

```

\end{lstlisting}

Please ensure you replace `process.env.UCP\_X\_API\_KEY` and `process.env.UCP\_BASE\_ENDPOINT` with your actual environment variable names if they differ.
