# Supplementary material for: APITestGenie: Automated API Test Generation through Generative AI
Source: arXiv:2409.03838 source file (2024-09-05)
Supplement: Supplementary file 3 [file appendix3.tex]

\chapter{Complex run generation}\label{apx:complexRun}

REQUIREMENT: As a user, I want to retrieve the price of accessories for a BMW car in the Italian market.

First test, using the `/vehicles` service, get a list of all available vehicle models in the market and select a random model. Second test, using the `/accessories` service and with the model previously selected, retrieve the list of all available accessories on the 17/05/2024. Third test, using the `/pricing` service to retrieve the calculated price of the available car accessories in the pcaso,con priceListsIdentifiers.

ENDPOINTS:

1) `/vehicles\censor{/sources/{source}/brands/{brand}/countries/{country}/models}`
    - Method: GET
    - Description: Retrieves a list of available BMW car models for a specific market.
    - Request Parameters: source, brand, country
    - Response: List of models with specific model codes.

2) `/accessories\censor{/channels/{channel}/countries/{country}/models/{modelCode}/validity-dates/{date}}`

    - Method: GET
    - Description: Fetches a list of all available accessories for a selected model code and a specific date.
    - Request Parameters: channel, country, modelCode, date
    - Response: List of accessories with details.

3) `/pricing\censor{/price-lists/{priceListsIdentifiers}/brands/{brand}/countries/{country}/effect-dates/{effectDate}/models/{modelCode}/available-accessories}`
    - Method: GET
    - Description: Gets the price of available accessories for a chosen model with prices valid for a specific date.
    - Request Parameters: priceListsIdentifiers, brand, country, effectDate, modelCode
    - Response: Prices of accessories including taxes and discounts, if any.

TEST:

\begin{lstlisting}[style=python]
```typescript
import axios from 'axios';

// Load environment variables
const API_KEY = process.env.UCP_X_API_KEY;
const BASE_ENDPOINT = process.env.UCP_BASE_ENDPOINT;

// Set common headers for axios
axios.defaults.headers.common[#\censor{'x-api-key'}#] = API_KEY;

describe('BMW Car Accessories Prices in Italian Market', () => {
  let selectedModelCode = '';

  test('Get a list of available BMW car models in the Italian market', async () => {
    const response = await axios.get(`${BASE_ENDPOINT}/vehicles#\censor{/sources/pcaso/ brands/bmwCar/countries/it/models}#`);
    expect(response.status).toBe(200);
    const models = response.data;
    expect(models).toBeDefined();
    const modelCodes = Object.keys(models);
    expect(modelCodes.length).toBeGreaterThan(0); // Ensure at least one model is available
    // Select a random model
    selectedModelCode = modelCodes[Math.floor(Math.random() * modelCodes.length )];
    expect(selectedModelCode).toBeTruthy();
  });

  test('Retrieve the list of all available accessories for the selected model on the 17/05/2024', async () => {
    const date = '2024-05-17';
    const response = await axios.get(`${BASE_ENDPOINT}/accessories#\censor{/channels/ con/countries/it/models/${selectedModelCode}/validity-dates/${date}}#`);
    expect(response.status).toBe(200);
    const accessories = response.data;
    expect(accessories).toBeDefined();
    expect(Object.keys(accessories).length).toBeGreaterThan(0); // Ensure at least one accessory is available
  });

  test('Retrieve the calculated price for the available car accessories', async () => {
    const effectDate = '2024-05-17';
    const response = await axios.get(`${BASE_ENDPOINT}/pricing#\censor{/price-lists/ pcaso,con/brands/bmwCar/countries/it/effect-dates/${effectDate}/models/${selectedModelCode}/available-accessories}# `);
    expect(response.status).toBe(200);
    const accessoryPrices = response.data;
    expect(accessoryPrices).toBeDefined();
    // Assuming the response contains a list of accessories with their prices
    Object.entries(accessoryPrices).forEach(([accessoryId, priceData]) => {
      expect(priceData).toHaveProperty('netPrice');
      expect(priceData).toHaveProperty('grossPrice');
      // Further assertions can be made based on the response structure...
    });
  });
});
```
\end{lstlisting}

This code block provides the example test cases as requested. It includes tests to get available car models, retrieve accessories for a selected model, and finally get the prices of these accessories.
