# Supplementary material for: APITestGenie: Automated API Test Generation through Generative AI
Source: arXiv:2409.03838 source file (2024-09-05)
Supplement: Supplementary file 4 [file appendix5.tex]

\chapter{Public Validation Runs}\label{apx:publicRuns}

\section{Cat Fact Run 1}

\subsection{Business Requirement}
As a user of the cat-themed educational app,   I want to receive a new and random cat fact every time I open the app or refresh the content,   so that I can learn fun and intriguing information about cats and stay engaged with the app.

\subsection{Generation}

REQUIREMENT: The business requirement is to ensure that the cat-themed educational app provides a new and random cat fact to the user every time the app is opened or its content is refreshed. The tests must verify that the 'Get Random Fact' API endpoint returns a random cat fact successfully and that the fact is indeed different (random) on subsequent requests.

ENDPOINTS: There are three key endpoints specified in the API documentation:

GET /breeds

Query Parameter: limit (integer, optional) to limit the number of results.
Response: An array of Breed objects on a 200 response.
GET /fact

Query Parameter: max\_length (integer, optional) to specify the maximum length of the returned fact.
Response: A CatFact object on a 200 response or a 404 error if a fact is not found.
GET /facts

Query Parameters: max\_length (integer, optional) for maximum length of returned fact, and limit (integer, optional) to limit the number of results.
Response: An array of CatFact objects on a 200 response.
To fulfill the business requirement, I will focus primarily on the GET /fact endpoint, since it returns a random fact which aligns with the requirement for providing a new fact every time the app is refreshed or opened.

TEST:
\begin{lstlisting}[style=python]
    ```typescript
    import axios from 'axios';
    import { v4 as uuidv4 } from 'uuid';
    
    describe('Cat Facts API - Random Fact Endpoint', () => {
      const baseEndpoint = process.env.CATFACT_BASE_ENDPOINT;
    
      test('Ensure that random cat fact is returned successfully', async () => {
        const response = await axios.get(`${baseEndpoint}/fact`);
        expect(response.status).toBe(200);
        expect(response.data).toHaveProperty('fact');
        expect(typeof response.data.fact).toBe('string');
      });
    
      test('Ensure that different cat facts are returned on subsequent requests', async () => {
        const firstResponse = await axios.get(`${baseEndpoint}/fact`);
        const secondResponse = await axios.get(`${baseEndpoint}/fact`);
    
        expect(firstResponse.status).toBe(200);
        expect(secondResponse.status).toBe(200);
        expect(firstResponse.data).toHaveProperty('fact');
        expect(secondResponse.data).toHaveProperty('fact');
        expect(firstResponse.data.fact).not.toEqual(secondResponse.data.fact);
      });
    
      test('Ensure that max_length parameter limits the length of the fact', async () => {
        const maxLength = 100;
        const response = await axios.get(`${baseEndpoint}/fact`, {
          params: { max_length: maxLength },
        });
    
        expect(response.status).toBe(200);
        expect(response.data).toHaveProperty('fact');
        expect(response.data.fact.length).toBeLessThanOrEqual(maxLength);
      });
    });
    ```
\end{lstlisting}

Please remember to replace process.env.CATFACT\_BASE\_ENDPOINT with the actual environment variable containing the base URL of the Cat Facts API before running the test.

\section{Cat Fact Run 2}

\subsection{Business Requirement}
As a user of the cat-themed educational app,   I want to receive a new and random cat fact every time I open the app or refresh the content,   so that I can learn fun and intriguing information about cats and stay engaged with the app.

\subsection{Generation}

REQUIREMENT: To accommodate the requirement for a cat-themed educational app user who wishes to receive a new and random cat fact each time they open or refresh the app, we need to test that the /fact API endpoint consistently provides a unique and random cat fact. This implies that each request to this endpoint should result in a response with a different cat fact to maintain user engagement with the app.

ENDPOINTS: The /fact endpoint is a GET request that allows an optional max\_length query parameter to limit the length of the returned fact. The endpoint responds with a JSON object containing the cat fact and its length. Based on the schema definition provided, the response will be of type CatFact which contains the properties fact (a string) and length (an integer).

GET /fact
Query Parameters:
max\_length (integer, optional): maximum length of the returned fact.
Response:
200: A CatFact object containing a random fact.
404: Fact not found.
TEST:

\begin{lstlisting}[style=python]
```typescript
import axios from 'axios';

// Define the base URL from the environment variable
const BASE_URL = process.env.CATFACT_BASE_ENDPOINT;

describe('Random Cat Fact Retrieval', () => {
  // Ensures that a random cat fact is received upon each request
  test('receives a new random cat fact on each request', async () => {
    // First request to get a random cat fact
    const response1 = await axios.get(`${BASE_URL}/fact`);
    expect(response1.status).toBe(200);
    expect(response1.data).toHaveProperty('fact');
    const firstFact = response1.data.fact;

    // Ensure there are pauses between requests to improve randomness assurance
    await new Promise(resolve => setTimeout(resolve, 1000));

    // Second request to check for a new random fact
    const response2 = await axios.get(`${BASE_URL}/fact`);
    expect(response2.status).toBe(200);
    expect(response2.data).toHaveProperty('fact');
    const secondFact = response2.data.fact;

    // Validate that the two facts are not the same, indicating randomness
    expect(firstFact).not.toBe(secondFact);
  });

  // Test to verify that the max_length query parameter limits the fact length
  test('respects the max_length parameter', async () => {
    const maxLength = 50; // Example max_length value
    const response = await axios.get(`${BASE_URL}/fact`, { params:
    { max_length: maxLength } });
    expect(response.status).toBe(200);
    expect(response.data).toHaveProperty('fact');

    // Validate the fact's length does not exceed the specified limit
    expect(response.data.fact).toHaveLength(response.data.length);
    expect(response.data.length).toBeLessThanOrEqual(maxLength);
  });
});
\end{lstlisting}

\section{Cat Fact Run 3}

\subsection{Business Requirement}
As a user of the cat-themed educational app,   I want to receive a new and random cat fact every time I open the app or refresh the content,   so that I can learn fun and intriguing information about cats and stay engaged with the app.

\subsection{Generation}

REQUIREMENT: The business requirement is to ensure that the user receives a fresh and random cat fact every time the educational app is launched or refreshed, providing engaging and informative content about cats.

ENDPOINTS: Here are the relevant endpoints from the API specification we'll need to test:

Get Random Fact (/fact - GET)

Request Query: max\_length (integer, optional)
Response: 200 with a CatFact schema object, 404 if fact is not found
Get a list of Facts (/facts - GET)

Request Query: max\_length (integer, optional), limit (integer, optional)
Response: 200 with an array of CatFact schema objects
The CatFact schema object consists of:

fact: string
length: integer
We will create tests to verify that a random cat fact can be retrieved successfully and that the content changes upon each request, thereby meeting the business requirement.

TEST:

\begin{lstlisting}[style=python]
```typescript
import axios from 'axios';

describe('Cat Facts API integration tests', () => {
  const BASE_ENDPOINT = process.env.CATFACT_BASE_ENDPOINT;

  test('should receive a random cat fact', async () => {
    // Call the random fact endpoint
    const randomFactResponse = await axios.get(`${BASE_ENDPOINT}/fact`);

    // Check that the response status is 200 and fact is received
    expect(randomFactResponse.status).toBe(200);
    expect(randomFactResponse.data.fact).toBeDefined();
    expect(typeof randomFactResponse.data.fact).toBe('string');

    // A random fact should have a non-zero length
    expect(randomFactResponse.data.length).toBeGreaterThan(0);
  });

  test('should receive a different random cat fact on a subsequent request', async () => {
    // Call the random fact endpoint twice
    const firstResponse = await axios.get(`${BASE_ENDPOINT}/fact`);
    const secondResponse = await axios.get(`${BASE_ENDPOINT}/fact`);

    // Check that both facts are defined
    expect(firstResponse.data.fact).toBeDefined();
    expect(secondResponse.data.fact).toBeDefined();

    // Check that the facts received are different
    expect(firstResponse.data.fact).not.toBe(secondResponse.data.fact);
  });

  test('should respect the maximum length of facts when provided', async () => {
    // Define the maximum length for the test
    const maxLength = 50;

    // Call the random fact endpoint with the maximum length
    const response = await axios.get(`${BASE_ENDPOINT}/fact`, {
      params: { max_length: maxLength }
    });

    // Check that the fact received respects the maximum length
    expect(response.data.fact.length).toBeLessThanOrEqual(maxLength);
  });

  // Add more tests for other scenarios if necessary...
});
\end{lstlisting}

\section{Pet Shop Run 1}

\subsection{Business Requirement}

Adding a New Pet to the Store Inventory As a pet store manager, I want to be able to add new pets to the store's inventory through the API, So that I can keep the store's inventory up-to-date and offer a wide variety of pets to our customers.

\subsection{Generation}

REQUIREMENT: Integrating a feature to add new pets to the store's inventory is crucial for maintaining an up-to-date offering for customers. The integration test must verify the functionality of the API endpoint responsible for adding new pet entries. The specific aspect this test is verifying is the API's ability to accept a valid pet object and successfully add it to the store's inventory, as well as handling invalid inputs appropriately.

ENDPOINTS: POST /pet - This endpoint is used to add a new pet to the store inventory. It requires a pet object as input and returns various HTTP status codes to indicate success or failure.

The pet object has the following structure:

id: integer (int64)
category: object with { id: integer (int64), name: string }
name: string
photoUrls: Array of strings
tags: Array of objects with { id: integer (int64), name: string }
status: string ['available', 'pending', 'sold']
The response will provide HTTP status code 405 if the input is invalid.

To set up the correct test environment state, the test script needs to generate a valid pet object that matches the expected schema for the API.

TEST:
\begin{lstlisting}[style=python]
```typescript
import axios from 'axios';

// Describe the feature being tested
describe('Pet Store Inventory - Add new pet', () => {
  const petStoreEndpoint = process.env.PETSHOP_BASE_ENDPOINT; // Load the environment variable

  // Test for adding a new valid pet to the inventory
  test('Add a new valid pet to the inventory', async () => {
    // Prepared test data with a valid pet object
    const newPetData = {
      id: 0, // 0 or a specific id value can be used if needed
      category: {
        id: 0, // Example category id
        name: "Dogs" // Example category name
      },
      name: "Rex", // Example pet name
      photoUrls: ["https://example.com/image.jpg"], // Example photo URL
      tags: [
        {
          id: 0, // Example tag id
          name: "Tag1" // Example tag name
        }
      ],
      status: "available" // Pet availability status
    };

    // Make request with generated data
    const response = await axios.post(`${petStoreEndpoint}/pet`, newPetData);

    // Validate that the response is successful
    expect(response.status).toBe(200); // Assuming 200 is the success status code
    expect(response.data).toMatchObject(newPetData); // This checks if the created pet matches the sent object
  });

  // Test for handling invalid input while adding a pet
  test('Attempt to add a pet with invalid data', async () => {
    // Prepared test data with an invalid pet object
    const invalidPetData = {
      // This object lacks the required 'name' and 'photoUrls' fields
      id: 0,
      category: {
        id: 0,
        name: "Dogs"
      },
      // name is missing
      // photoUrls is missing
      tags: [
        {
          id: 0,
          name: "Tag1"
        }
      ],
      status: "available"
    };

    // Expecting axios to throw an error on the invalid request
    await expect(axios.post(`${petStoreEndpoint}/pet`, invalidPetData))
    .rejects.toHaveProperty('response.status', 405);
  });
});
\end{lstlisting}

\section{Pet Shop Run 2}

\subsection{Business Requirement}

Adding a New Pet to the Store Inventory As a pet store manager, I want to be able to add new pets to the store's inventory through the API, So that I can keep the store's inventory up-to-date and offer a wide variety of pets to our customers.

\subsection{Generation}

REQUIREMENT: The business requirement is to develop an integration test that validates the ability to add a new pet to the store's inventory through an API endpoint. This ensures that the pet store manager can update the store's inventory, reflecting the introduction of new pets for customers to purchase.

ENDPOINTS: The relevant endpoint from the API specification for adding a new pet to the store's inventory is:

POST /pet
Operation: addPet
Request Body: Object of type Pet (required)
Responses:
405: Invalid input
In order to perform a valid test, we must ensure that the request conforms to the Pet object's structure described in the specification. This includes attributes like id, name, photoUrls, and optional elements like category, tags, and status.

TEST:

\begin{lstlisting}[style=python]
```typescript
import axios from 'axios';
import { Pet } from './models/Pet'; // Hypothetically importing Pet type from models

const PETSHOP_BASE_ENDPOINT = process.env.PETSHOP_BASE_ENDPOINT ||
"https://petstore.swagger.io/v2";

describe('Petstore API - Add New Pet Integration Test', () => {
  test('It should add a new pet to the inventory', async () => {
    const newPet: Pet = {
      id: 0, // This will likely be auto-generated by the server on actual entry
      name: 'Goldie',
      photoUrls: ['http://example.com/photo_of_goldie.jpg'],
      status: "available"
      // Optional fields like 'tags' and 'category' can be added if required
    };

    try {
      // Creating a new pet
      const response = await axios.post(`${PETSHOP_BASE_ENDPOINT}/pet`, newPet);

      // The response status code for successful pet creation should be checked against the API documentation
      // Assuming 200 is the success code for pet creation which isn't specified in the provided spec
      expect(response.status).toBe(200); 

      // Verify that the response body matches the pet that was sent
      expect(response.data.name).toBe(newPet.name);
      expect(response.data.photoUrls).toEqual(newPet.photoUrls);
      expect(response.data.status).toBe(newPet.status);

      // Confirm that the ID has been generated for the new pet
      expect(response.data.id).toBeDefined();

      // Check for other properties that should be returned in a successful creation
      // e.g., category and tags if they are included in the newPet object
    } catch (error) {
      if (axios.isAxiosError(error) && error.response) {
        // We may want to output additional information here for debug purposes
        console.error('API responded with status code:', error.response.status);
        console.error('Response body:', error.response.data);
      } else {
        console.error('An unexpected error occurred:', error);
      }
      throw error; // Re-throw the error to fail the test if the API call was not successful
    }
  });
});
\end{lstlisting}

Note: The Pet type used in the test code would typically be defined according to the API's contract. Since the actual API specification might include additional optional or required fields, the Pet type should be defined accordingly to match the specification. The model import path should be adjusted based on the project's actual structure.

\section{Pet Shop Run 3}

\subsection{Business Requirement}

Adding a New Pet to the Store Inventory As a pet store manager, I want to be able to add new pets to the store's inventory through the API, So that I can keep the store's inventory up-to-date and offer a wide variety of pets to our customers.

\subsection{Generation}

REQUIREMENT: Adding a New Pet to the Store Inventory requires an API endpoint that allows the pet store manager to post new pet data to the store's inventory. The test should verify that upon submitting a well-formed pet object to the designated endpoint, the server processes the request appropriately and adds the new pet to the inventory.

ENDPOINTS: The relevant endpoint for this requirement is: POST /pet

This endpoint accepts a new pet object and adds it to the store. The request must contain a pet object in the request body. The pet object includes a required name and photoUrls, along with optional fields such as id, category, tags, and status.
The types for request and response objects are as follows:

Request Object (Pet):

id (integer, optional)
category (object, optional)
id (integer, optional)
name (string, optional)
name (string, required)
photoUrls (array of strings, required)
tags (array of objects, optional)
id (integer, optional)
name (string, optional)
status (string, optional) - Enum:['available', 'pending', 'sold']
Response:

The response body should contain the newly added Pet object.
HTTP Status codes:
200 OK for a successful addition of a pet,
405 Method Not Allowed if invalid input is provided.
TEST:

\begin{lstlisting}[style=python]
```typescript
import axios from 'axios';

// Define the base URL from the environment variable
const BASE_URL = process.env.PETSHOP_BASE_ENDPOINT;

describe('Pet Store Inventory - Add New Pet API Test', () => {
   test('It should successfully add a new pet to the inventory', async () => {
     // Prepared test data
     const newPet = {
       name: 'Fluffy',
       photoUrls: ['http://example.com/photos/fluffy.jpg'],
       status: 'available'
     };

     try {
       // Make request to add new pet
       const response = await axios.post(`${BASE_URL}/pet`, newPet);

       // Validate response status code
       expect(response.status).toBe(200);

       // Assert response body
       expect(response.data.name).toBe(newPet.name);
       expect(response.data.photoUrls).toEqual(
        expect.arrayContaining(newPet.photoUrls));
       expect(response.data.status).toBe(newPet.status);

       // Additional check could be made to retrieve the pet using GET /pet/{petId} and validate that it is in the inventory
     } catch (error) {
       // If the request fails, log the response for debugging purposes
       console.error('API request failed with response:', error.response);
       // Rethrow the error for Jest to fail the test
       throw error;
     }
   });

   test('It should reject adding a new pet with incomplete data', async () => {
     // Prepared test data with missing required fields (photoUrls)
     const incompletePet = {
       name: 'Ghost'
     };

     try {
       // Attempt to add incomplete pet
       await axios.post(`${BASE_URL}/pet`, incompletePet);
     } catch (error) {
       // Validate response status code
       expect(error.response.status).toBe(405);

       // Assert the response body to contain a meaningful error message
       // Note: This assertion depends on the API's implementation of error messages, which might be different
       // expect(error.response.data.message).toMatch(/invalid input/i);
     }
   });
});
\end{lstlisting}

Please make sure you replace the process.env.PETSHOP\_BASE\_ENDPOINT with the actual URL when running the test.

\section{Pet Shop Run 4}

\subsection{Business Requirement}

Title: Create New User Description: As a client of the pet store application, I want to be able to create a new user account, so that I can access and use the various features and functionalities of the application.

\subsection{Generation}

REQUIREMENT: The business requirement is to validate the capability to create a new user account on the pet store application so that the user can access various features and functionalities of the application.

ENDPOINTS: For creating a new user, the endpoint that will be used is:

POST /user
Request Object: User
id (integer, int64)
username (string)
firstName (string)
lastName (string)
email (string)
password (string)
phone (string)
userStatus (integer, int32)
Response Object: usually empty with HTTP status indicating success (200 OK) or failure.
TEST:

\begin{lstlisting}[style=python]
```typescript
import axios from 'axios';

// Assign the base endpoint for the API requests to a variable
const PETSHOP_BASE_ENDPOINT = process.env.PETSHOP_BASE_ENDPOINT || 
'https://petstore.swagger.io/v2';

describe('Create New User Endpoint', () => {
  test('It should create a new user account', async () => {
    // Data for a new user account
    const newUser = {
      username: 'newUser',
      firstName: 'John',
      lastName: 'Doe',
      email: 'johndoe@example.com',
      password: 'securePassword123',
      phone: '123-456-7890',
      userStatus: 1 // Assuming '1' stands for active user
    };

    // Execute the API call to create a new user
    const response = await axios.post(`${PETSHOP_BASE_ENDPOINT}/user`, newUser);

    // Evaluate the response to ensure the user creation was successful
    expect(response.status).toBe(200);

    // If the API returns additional data on user creation, like a user object or id
    // additional assertions can be made here, such as:
    // expect(response.data.id).toBeDefined();
    // expect(response.data.username).toBe(newUser.username);
  });

  // You can add more tests, for instance, a negative test to check if creating a user with an existing username fails
  // or whether the required fields are correctly validated by the API.
});
\end{lstlisting}

\section{Pet Shop Run 5}

\subsection{Business Requirement}

Title: Create New User Description: As a client of the pet store application, I want to be able to create a new user account, so that I can access and use the various features and functionalities of the application.

\subsection{Generation}

REQUIREMENT: To ensure that clients have the ability to create new user accounts in the pet store application, there is a need to validate the functionality of the user account creation API endpoint. The test will verify the API's ability to accept the creation of new user accounts and return a successful response indicating that the user account has been created.

ENDPOINTS: The specific endpoint involved in the creation of a new user account is:

POST /user: This endpoint expects a request body that adheres to the User object structure and will return a default successful operation response upon the successful creation of a new user account.
A valid User object includes the following fields: id (integer), username (string), firstName (string), lastName (string), email (string), password (string), phone (string), and userStatus (integer).

The response structure is not specified in detail, but a successful user creation results in a default success message.

TEST:
\begin{lstlisting}[style=python]
```typescript
import axios from 'axios';

describe('User Account Creation', () => {
  const baseUrl = process.env.PETSHOP_BASE_ENDPOINT;

  test('Create a new user account', async () => {
    // Prepared test data
    const userData = {
      id: 0,
      username: 'new_user',
      firstName: 'John',
      lastName: 'Doe',
      email: 'johndoe@example.com',
      password: 'password123',
      phone: '123-456-7890',
      userStatus: 1
    };

    // Setup test environment
    // In this case, no additional setup is needed.

    // Make request with generated data
    const response = await axios.post(`${baseUrl}/user`, userData);

    // Validate response of request
    // Since the API specification doesn't provide a specific success response schema,
    // we check for a successful HTTP response status code.
    expect(response.status).toBe(200);

    // For a more robust test, you might query the `/user/{username}` endpoint
    // to verify the new user was indeed created and matches the submitted data.
  });

  // Additional tests could include:
  // - attempting to create a user with existing username (expect failure response)
  // - creating a user with incomplete data (expect failure response)
  // - validating server response for malformed user data (expect failure response)
});
\end{lstlisting}

Please note that before running the test, you have to set the PETSHOP\_BASE\_ENDPOINT environment variable to point to the base URL of your pet store API (e.g. http://petstore.swagger.io/v2).

\section{Pet Shop Run 6}

\subsection{Business Requirement}
Title: Create New User Description: As a client of the pet store application, I want to be able to create a new user account, so that I can access and use the various features and functionalities of the application.

\subsection{Generation}

REQUIREMENT: In order to test the ability to create a new user account within the pet store application, the integration test must ensure that a user object can be submitted to the relevant API endpoint, and that the endpoint successfully creates a user with the provided details.

ENDPOINTS: The endpoint used for this operation is:

POST /user
Request object type: User
Response object should be a successful operation message (no specific structure is described for a successful creation in the API specification, so it should just not return an error response such as 400 or 404).
TEST:

\begin{lstlisting}[style=python]
```typescript
import axios from 'axios';
import { User } from './types'; // Assume types are defined as per the API's swagger definitions

// The base endpoint URL from the Swagger pet store API
const BASE_URL = process.env.PETSHOP_BASE_ENDPOINT || 
'https://petstore.swagger.io/v2';

describe('User account creation', () => {
  test('Successfully creates a new user', async () => {
    // User data to create a new user
    const userData: User = {
      id: 0, // Assume the ID is generated by the server
      username: 'john_doe',
      firstName: 'John',
      lastName: 'Doe',
      email: 'johndoe@example.com',
      password: 'password123',
      phone: '123-456-7890',
      userStatus: 1 // assuming 1 indicates active user
    };

    // Define the URL for user creation endpoint
    const createUserUrl = `${BASE_URL}/user`;

    // Make request to create a new user
    const response = await axios.post(createUserUrl, userData);

    // Validate response to ensure success status code (usually 200)
    expect(response.status).toBe(200);

    // We would ideally have something to check in the response body to confirm the user was created,
    // such as a 'message' or 'id' field, but since the specification does not detail the response
    // body for this endpoint, we can only really check that it didn't return an error.
    // Additional verification could be done by calling a GET endpoint if that were available and in scope.
  });

  // Here you could add more tests for scenarios like user creation with existing username or bad input
});
\end{lstlisting}
