# Supplementary material for: APITestGenie: Automated API Test Generation through Generative AI
Source: arXiv:2409.03838 source file (2024-09-05)
Supplement: Supplementary file 5 [file appendix4.tex]

\chapter{No code generation}\label{apx:noCode}

REQUIREMENT: Unfortunately, there is no specific business requirement provided in the narrative. Without a specific requirement, endpoints cannot be selected for testing nor can valid assertions be made about their behavior. If you have a specific business requirement that needs to be tested, please provide it, and I will create the relevant API integration tests.

ENDPOINTS: Since no specific endpoints are requested to be tested based on a business requirement, I cannot list endpoints that the test script will interact with. Should you have certain endpoints in mind that need to be tested, please specify, and I will include them in the testing process along with the respective request and response objects.

TEST: Without clear instructions or a specific business requirement to validate against API endpoints, generating executable test code is not possible. If detailed requirements and endpoints for testing are provided, I will gladly supply the TypeScript code using Axios and Jest to create integration tests.
